# Supplementary material for: Complexity Analysis of Tree Share Structure
Source: arXiv:2010.02340 source file (2020-10-05)
Supplement: Supplementary file 1 [file appendix.tex]

\lstset{%
  language=C,
  backgroundcolor=\color{white},
  morecomment=[n][{\commentcolor}]{/*}{*/},
  morecomment=[l][{\commentcolor}]{//},
  sensitive=true,
  mathescape=true,
  showlines=true,
  basicstyle=\tt,
  keywordstyle=\color{red}, %\color{BrickRed},
  numbers=left,
  numberstyle=\tiny,
  numbersep=5pt,
  boxpos=t
}
\def \fperm {\ensuremath{\mathcal{F}}}
\def \eperm {\ensuremath{\mathcal{E}}}
\newcommand{\p}[1]{\ensuremath{\mathsf{#1}}}
\newcommand{\m}[1]{\ensuremath{\mathit{#1}}}
\newcommand{\commentcolor}{\color{blue}}

\newcommand{\tx}[1]{\ensuremath{\mathtt{#1}}}
\def \lshare{\ensuremath{\mathcal{L}}}
\def \rshare{\ensuremath{\mathcal{R}}}
\def \hmul {\ensuremath{\cdot}}

\section{Application of tree shares in program verification}\label{sec:appendix}
\begin{figure}
%\lstset{numbers=none}
\begin{lstlisting}[name=example1code]
struct tree {int d; struct tree* l; struct tree* r;};
void processTree(struct tree* x) { $\label{code:toystart}$
  if (x == 0) { return; } $\label{code:toyifnull}$
\end{lstlisting}
\vspace{-1em}
\begin{tabular}{@{}l@{}||@{\hspace{1em}}l@{}}
\begin{minipage}{0.40\textwidth}
\begin{lstlisting}[name=example1code]
  print(x -> d); $\label{code:toypara1start}$
  processTree(x -> l); $\label{code:toypara1mid}$
  processTree(x -> r); $\label{code:toypara1end}$
\end{lstlisting}
\end{minipage} &
\begin{minipage}{0.40\textwidth}
\begin{lstlisting}[name=example1code]
  print(x -> d); $\label{code:toypara2start}$
  processTree(x -> l); $\label{code:toypara2mid}$
  processTree(x -> r); $\label{code:toypara2end}$
\end{lstlisting}
\end{minipage}
\vspace{-0.75em}
\end{tabular}
\begin{lstlisting}[name=example1code]
} $\label{code:toyend}$
\end{lstlisting}
%\lstset{numbers=left}
\vspace{-1em}
\caption{The parallel \texttt{processTree} function, written in a C-like language}
\vspace{-1.5em}
\label{fig:processtree}
\end{figure}

Consider the toy program in Figure~\ref{fig:processtree} which is taken from~\cite{le17:logic}.
Starting from the tree rooted at \texttt{x}, the program itself is extremely 
simple.  First (line~\ref{code:toyifnull})
we check if the \texttt{x} is null, \emph{i.e.} if we have reached a leaf; if so, we \texttt{return}.  If not, we split into parallel threads (lines $\ref{code:toypara1start}$--$\ref{code:toypara1end}$ and $\ref{code:toypara2start}$--$\ref{code:toypara2end}$) that do some processing on the root data in both branches.  In the toy example, the processing just \texttt{print}s out the root data (lines $\ref{code:toypara1start}$ and $\ref{code:toypara2start}$); the \texttt{print} command is unimportant: what is important that we somehow access some of the data in the tree.  After processing the root, both parallel branches call the \texttt{processTree} function recursively on the left \texttt{x->l} (lines \ref{code:toypara1mid} and \ref{code:toypara2mid}) and right \texttt{x->r} (lines \ref{code:toypara1end} and \ref{code:toypara2end}) branches, respectively.  After both parallel processes have terminated, the function returns (line \ref{code:toyend}).  The initial caller (unshown) may then \emph{e.g.} deallocate the tree.  The program is simple, so we would like its verification to be equally simple.

Predicate multiplication is the tool that leads to a simple proof.  Specifically, we would like to verify that \texttt{processTree} has the specification:
\vspace{-1.5ex}
$$
\forall \pi,x. ~~\big(~ \{\pi \cdot \p{tree}(x)\} ~~ {\color{black}\tt{processTree(} \m{x} \tt{)}} ~~ \{\pi \cdot \p{tree}(x)\}~\big). 
\vspace{-0.5ex}
$$
where the $\p{tree}$ predicate is defined recursively:
$$
\p{tree}(x) ~\defi~ (x = 0) \vee \exists d,l,r.~x \xmapsto{\fperm} (d,l,r) \star \p{tree}(l) \star \p{tree}(r) .
$$

Our precondition and postcondition both say that $x$ is a pointer to a heap-represented $\pi$-owned \p{tree}.  Critically, we want to ensure that our $\pi$-share at the end of the program is equal to the $\pi$-share at the beginning.  This way if our initial caller had full ownership before calling \texttt{processTree}, he will have full ownership afterwards (allowing him to \emph{e.g.} deallocate the tree). For convenience, we will use the letter $\fperm$ for $\bullet$, $\eperm$ for $\circ$, $\lshare$ for $\Tree[ $\bullet$ $\circ$ ]$ and $\rshare$ for $\Tree[ $\circ$ $\bullet$ ]$. Also, we define the share multiplication $\otimes$ as reversed bowtie, \emph{i.e.}
$$
\pi_1 \otimes \pi_2 = \pi_3 \defi \pi_2 \bowtie \pi_1 = \pi_3 .
$$

In Figure~\ref{fig:bigexample} we put the formal verification for \texttt{processTree} whose intuition is as follow.  First in line~\ref{code:toyifnull}, we check if \tx{x} is null; if so we are in the base case of the \p{tree} definition and can simply return.  If not we can eliminate the left disjunct and can proceed to split the $\star$-separated bits into disjoint subtrees $\tx{l}$ and $\tx{r}$, and then dividing the ownership of those bits into two ``halves'' $\lshare$ and $\rshare$. When we start start the parallel computation on lines \ref{code:toypara1start} and \ref{code:toypara2start} we want to pass the left branch of the computation the $\lshare \otimes \pi$-share of the spatial resources, and the right branch of the computation the $\rshare \otimes \pi$.  In both branches we then need to show that we can read from the data cell, which in the simple policy we use for this paper boils down to making sure that the product of two non-$\eperm$ shares cannot be $\eperm$.  This is a basic property for reasonable share models with multiplication.  In the remainder of the parallel code (lines \ref{code:toypara1mid}--\ref{code:toypara1end} and \ref{code:toypara2mid}--\ref{code:toypara2end}) we need to make recursive calls, which is done by simply instantiating $\pi$ with $\lshare \otimes \pi$ and $\rshare \otimes \pi$ in the recursive specification (as well as \tx{l} and \tx{r} for $x$). The later half proof after the parallel call is pleasantly symmetric to the first half in which we fold back the original tree predicate by merging the two halves $\lshare \otimes \pi$ and $\rshare \otimes \pi$ back into $\pi$. Consequently, we arrive at the postcondition $\pi \hmul \textsf{tree}(x)$, which is identical to the precondition. Curious readers are invited to read the full explanation together with formal proof rules in~\cite{le17:logic}.

\begin{figure}
\begin{lstlisting}[name=example1]
void processTree(struct tree* x) { // $\label{code:startverif}\codecomment{~\pi \cdot \p{tree}(\tx{x})~}$
// $\label{code:unfoldtree}\codecomment{ \begin{array}{@{}l@{}l@{}}  \pi \cdot \Big( & \big\langle\tx{x} = \texttt{null} \big\rangle ~\vee~ \null \big(\exists d,l,r.~\tx{x} \mapsto (d,l,r) ~\star~ \p{tree}(l) ~\star~ \p{tree}(r) \big) \Big) \end{array} }$
// $\label{code:pushdotin}\codecomment{ \begin{array}{@{}l@{}l@{}} & \Big\langle\tx{x} = \texttt{null} \Big\rangle ~\vee~ \null \Big( \exists d,l,r.~ \tx{x} \stackrel{\pi}{\mapsto} (d,l,r) ~\star~ \big(\pi \cdot \p{tree}(l)\big) ~\star~ \big(\pi \cdot \p{tree}(r)\big) \Big) \end{array} }$
  if (x == null) { // $\label{code:inif}\codecomment{ \langle\tx{x} = \texttt{null} \rangle }$
  return;} // $\label{code:endif}\codecomment{~\pi \cdot \p{tree}(\tx{x})~}$ 
// $\label{code:afterif}\codecomment{ \begin{array}{@{}l@{}l@{}} \tx{x} \stackrel{\pi}{\mapsto} (d,l,r) ~\star~ \big(\pi \cdot \p{tree}(l)\big) ~\star~ \big(\pi \cdot \p{tree}(r)\big) \end{array} }$
// $\label{code:mulF}\codecomment{ \begin{array}{@{}l@{}l@{}} \fperm \cdot \Big( \tx{x} \stackrel{\pi}{\mapsto} (d,l,r) ~\star~ \big(\pi \cdot \p{tree}(l)\big) ~\star~ \big(\pi \cdot \p{tree}(r)\big) \Big) \end{array} }$
// $\label{code:splitF}\codecomment{ \begin{array}{@{}l@{}l@{}} (\lshare \oplus \rshare) \cdot \Big(\tx{x} \stackrel{\pi}{\mapsto} (d,l,r) ~\star~ \big(\pi \cdot \p{tree}(l)\big) ~\star~ \big(\pi \cdot \p{tree}(r)\big) \Big) \end{array} }$
// $\label{code:distribF}\codecomment{ \begin{array}{@{}l@{}l@{}} \Big(\mathcal{L} & \cdot \Big(\tx{x} \stackrel{\pi}{\mapsto} (d,l,r) ~\star~ \big(\pi \cdot \p{tree}(l)\big) ~\star~ \big(\pi \cdot \p{tree}(r)\big) \Big) \Big) ~\star~ \null \\ \Big(\mathcal{R} & \cdot \Big( \tx{x} \stackrel{\pi}{\mapsto} (d,l,r) ~\star~ \big(\pi \cdot \p{tree}(l)\big) ~\star~ \big(\pi \cdot \p{tree}(r)\big) \Big) \Big) \end{array} }$
\end{lstlisting} \vspace{-0.65em}
\begin{tabular}{@{}l||l}
\begin{minipage}{0.8\textwidth}
\begin{lstlisting}[name=example1]
// $\label{code:startpara}\codecomment{ \begin{array}{@{}l@{}l@{}} \mathcal{L} \cdot \Big(\tx{x} \stackrel{\pi}{\mapsto} (d,l,r) ~\star~ \big(\pi \cdot \p{tree}(l)\big) ~\star~ \big(\pi \cdot \p{tree}(r)\big) \Big) \end{array} }$
// $\label{code:parapushin}\codecomment{ \begin{array}{@{}l@{}l@{}} \mathcal{L} \cdot \tx{x} \stackrel{\pi}{\mapsto} (d,l,r) ~\star~ \mathcal{L} \cdot \pi \cdot \p{tree}(l) ~\star~ \mathcal{L} \cdot \pi \cdot \p{tree}(r) \end{array} }$
// $\label{code:paradotin}\codecomment{ \begin{array}{@{}l@{}l@{}} \tx{x} \stackrel{\mathcal{L} \otimes \pi}{\longmapsto} (d,l,r) ~\star~ \big((\mathcal{L} \otimes \pi) \cdot \p{tree}(l)\big) ~\star~ \big((\mathcal{L} \otimes \pi) \cdot \p{tree}(r)\big) \end{array} }$
  print(x -> d); $\label{code:print}$ 
  processTree(x -> l); $\label{code:reccall}$ processTree(x -> r); $\label{code:reccalr}$
// $\label{code:aftertreeframe}\codecomment{ \begin{array}{@{}l@{}l@{}} \tx{x} \stackrel{\mathcal{L} \otimes \pi}{\longmapsto} (d,l,r) ~\star~ \big((\mathcal{L} \otimes \pi) \cdot \p{tree}(l)\big) ~\star~ \big((\mathcal{L} \otimes \pi) \cdot \p{tree}(r)\big) \end{array} }$
// $\label{code:pullout}\codecomment{ \begin{array}{@{}l@{}l@{}} \mathcal{L} \cdot \pi \cdot \tx{x} \mapsto (d,l,r) ~\star~ \mathcal{L} \cdot \pi \cdot \p{tree}(l) ~\star~ \mathcal{L} \cdot \pi \cdot \p{tree}(r) \end{array} }$
// $\label{code:endpara}\codecomment{ \begin{array}{@{}l@{}l@{}} \mathcal{L} \cdot \pi \cdot \big(\tx{x} \mapsto (d,l,r) ~\star~ \p{tree}(l) ~\star~ \p{tree}(r) \big) \end{array} }$
\end{lstlisting} \end{minipage} & \ldots
\end{tabular}
\vspace{-1em}
\begin{lstlisting}[name=example1]
// $\label{code:afterpara}\codecomment{ \begin{array}{@{}l@{}l@{}} \Big(\mathcal{L} & \cdot \pi \cdot \big(\tx{x} \mapsto (d,l,r) ~\star~ \p{tree}(l) ~\star~ \p{tree}(r) \big) \Big) ~\star~ \null \\ \Big(\mathcal{R} & \cdot \pi \cdot \big(\tx{x} \mapsto (d,l,r) ~\star~ \p{tree}(l) ~\star~ \p{tree}(r) \big) \Big) \end{array} }$
// $\label{code:plusdotin}\codecomment{ \begin{array}{@{}l@{}l@{}} (\mathcal{L} \oplus \mathcal{R}) \cdot \pi \cdot \big(\tx{x} \mapsto (d,l,r) ~\star~ \p{tree}(l) ~\star~ \p{tree}(r) \big)\Big) \end{array} }$
} // $\label{code:endverif}\codecomment{~\pi \cdot \p{tree}(\tx{x})~}$
\end{lstlisting}
\vspace{-1em}
\caption{Reasoning with the scaling operator $\pi \cdot P$.}
\vspace{-1em}
\label{fig:bigexample}
\end{figure}

Note that if we want to jump directly from line 6 to line 9 in Figure~\ref{fig:bigexample} then the following tree share property needs to be checked by share solver:
$$
\forall \pi.~\pi = \pi \bowtie (\lshare \oplus \rshare).
$$

Alternatively, the inferences between lines $6 \rightarrow 7$, $7 \rightarrow 8$, $8 \rightarrow 9$ require these properties of tree shares respectively:
\begin{enumerate}
\item $\forall \pi.~\pi = \pi \bowtie \fperm$
\item $\fperm = \lshare \oplus \rshare$
\item $\forall \pi.~\pi\bowtie(\lshare \oplus \rshare) = (\pi \bowtie \lshare) \oplus (\pi \bowtie \rshare)$.
\end{enumerate}

As a result, share solver need to be able to reason about formulas with both $\oplus$ and $\bowtie$ in which the second operand of $\bowtie$ is constant.
